# Supplementary material for: Sparse species interactions reproduce abundance correlation patterns in microbial communities
Source: arXiv:2305.19154 ancillary file (2023-12-06)
Supplement: Supplementary file 1 [file SupplementaryMaterial.pdf]

# Species interactions reproduce abundance correlations patterns in microbial communities

## Supporting Information

José Camacho-Mateu, Aniello Lampo, Matteo Sireci, Miguel Ángel Muñoz, José A. Cuesta

## S1 Simulation of *in silico* communities

We model the population dynamics of species $i = 1, \dots, S$ in a microbial community as:

$$\dot{x}_i(t) = \frac{x_i(t)}{\tau_i}\left(1 + \sum_{j=1}^{S} a_{ij}x_j(t)\right) + x_i(t)\xi_i(t), \tag{S1}$$

where $x_i(t)$ represents the population (also called abundance or density of individuals) of species $i$, $\tau_i$ is the corresponding time scale of basal population growth, and $\xi_i(t)$ is a zero-mean Gaussian white noise with correlations $\langle\xi_i(t)\xi_j(t')\rangle = w_{ij}\delta(t - t')$. The matrix $\mathbf{W} = (w_{ij})$ accounts for correlations in the environmental fluctuations sensed by diverse species, whereas the off-diagonal terms of matrix $\mathbf{A} = (a_{ij})$ describe direct, Lotka-Volterra-like direct interactions between species, and the diagonal terms $a_{ii} = -1/K_i$ incorporate the carrying capacities of the environment. We will refer to this model as the Stochastic Lotka-Volterra Model (SLVM).

Equation (S1) is solved numerically using an Euler-Maruyama integration scheme [1]. The simulations presented in the paper span a time interval $0 \leq t \leq 10$, with a typical integration time step $\Delta t = 0.01$. Simulations performed using different time steps yield similar results. For each species, the solution represents a noisy trajectory fluctuating around some stationary-state population, which is determined by interactions, as shown in Fig. S1. Information about the statistics of the population is sampled in two different ways:

- **Longitudinal data**: We run the dynamics (S1) with one initial condition and sample the trajectory at $N_c$ separated times, once the stationary state is reached (Fig. S2 left). Time spacing between samples is large enough to avoid autocorrelations.
- **Cross-sectional data**: We run (S1) $N_c$ times starting from the same initial condition, wait until the stationary state has been reached, and sample the abundances of all $N_c$ trajectories of a given species at the same time instant $t$ (Fig. S2 right)

The results presented in the paper have been obtained with $N_c = 100$, but are largely independent of this choice (for larger values of $N_c$). Both longitudinal and cross-sectional data lead to the same macroecological patterns, which means that the dynamic (S1) is ergodic.

At this stage, one may construct the table of data shown in Fig. S3**b**, *i.e.* a matrix whose rows are species and whose columns are samples. Element $(i, s)$ of this matrix contains the abundance of species $i$ in sample $s$. This is the basic structure connecting the population dynamics to the macroecological laws, as sketched in Fig. S4. Specifically, Fig. S5 depicts how the abundance fluctuation distribution (AFD) can be obtained in this framework. Similarly, Figs. S6 and S7 show how to recover the Taylor's law and the "Mean Abundance Distribution" (MAD), respectively.

## S2 Interactions affect the average abundances of the species

The SLVM (S1) with noise matrix $\mathbf{W} = w\mathbf{I}$ becomes

$$\dot{x}_i = \frac{x_i}{\tau_i}\left(1 + \sum_{j=1}^{S} a_{ij}x_j\right) + \sqrt{w}x_i\xi_i(t), \quad i = 1, \dots, S, \tag{S2}$$

where $\xi(t)$ is a zero-mean, Gaussian white noise with $\langle \xi_i(t)\xi_j(t')\rangle = \delta_{ij}\delta(t-t')$. We can use Itô's calculus to obtain

$$\frac{d}{dt}\log x_i = \frac{\dot{x}_i}{x_i} - \frac{w}{2} = \frac{1}{\tau_i}\left(1 + \sum_{j=1}^{S} a_{ij}x_j\right) - \frac{w}{2} + \sqrt{w}\xi_i(t), \tag{S3}$$

and averaging this equation,

$$\frac{d}{dt}\overline{\log x_i} = \frac{1}{\tau_i}\left(1 + \sum_{j=1}^{S} a_{ij}\bar{x}_j\right) - \frac{w}{2}, \tag{S4}$$

and given that in the stationary state the left-hand side is zero and therefore

$$\frac{w\tau_i}{2} = 1 + \sum_{j=1}^{S} a_{ij}\bar{x}_j. \tag{S5}$$

Therefore, this equation determines the mean values of the abundances as a function of matrix $\mathbf{A}$, growth rates $\tau_i^{-1}$, and $w$.

When $\mathbf{A}$ is a diagonal matrix we recover the Stochastic Logistic Model (SLM) [2] and then

$$\bar{x}_j^{\text{SLM}} = \left(1 - \frac{w\tau_i}{2}\right)K_i, \tag{S6}$$

so Grilli's third empirical law (a lognormal mean abundance distribution, which means that, on average, most species have low abundances, while a few of them have very large ones) can be imposed by just sampling the carrying capacities $K_i$ from a lognormal distribution. Equation (S5) though shows that a proper choice of the interaction constants may induce a lognormal distribution of the mean abundances even if the carrying capacities are all equal. This suggests a possible alternative origin of this third law, based on the structure and interactions of the network.

## S3 Feasibility and stability of *in silico* communities

Equation (S6) puts constraints on the matrices $\mathbf{A}$ that are suitable to model a microbial community. To begin with, the community must be *feasible*, meaning that $\bar{x}_i > 0$ for all $i = 1, ..., S$ [3, 4]. In the limit $w\tau_i/2 \ll 1$ (which holds for all the results in the main text), feasibility is determined solely by interactions. Actually, we can create a large sample of interaction matrices $\mathbf{A}$ by setting the diagonals to $a_{ii} = -K_i^{-1}$, with the carrying capacities $K_i$ drawn from a lognormal distribution $\log K_i \sim \mathcal{N}(\mu_{LN}, \sigma_{\text{LN}})$, and a fraction $C$ (connectance) of the off-diagonal constants $a_{ij}$ are drawn from a normal distribution $a_{ij} \sim \mathcal{N}(0, \sigma)$—while the rest are set to 0. From this sample of $\mathbf{A}$ matrices, we can estimate the probability that they lead to a feasible community by calculating the fraction of them that produce $\bar{x}_i > 0$ for all $i = 1, \dots, S$. The results are plotted in Fig. S9 as a function of $\sigma_{\text{LN}}$ and $\sigma$. This figure reveals that feasible communities can be obtained over a very wide range of parameters.

Natural communities do continuously experience variations, due to both extrinsic environmental conditions and intrinsic demographic/dynamical factors. The analysis of such variations and their influence on ecosystem stability is a crucial issue in community ecology. Specifically, during the last decades there has been a large profusion of

metrics aimed to assess stability [8]. Here, we focus on local asymptotic stability (hereafter stability), defined as the system's ability to restore the steady state after an infinitesimal perturbation of the abundances.

In the framework of (S1), the aforementioned notion of stability implies that smalls perturbations—e.g. those induced by the environmental stochastic noise $\xi(t)$—do not affect the stationary average abundances. In formal terms, this may be evaluated by looking at the spectral properties of the Jacobian matrix and, in particular, the sign of the largest real part of its eigenvalues, $\lambda_J^* = \max_{k=1,\dots,S} \mathrm{Re}(\lambda_k)$, which quantifies the linear long-term response of the equation to first-order perturbations of $x(t)$ —-if $\lambda_J^* < 0$ the system is meant to be stable, otherwise unstable.

The definition of the Jacobian depends in general on species populations and involves a large number of parameters. The effect of those populations on the analysis of stability has been carefully studied, both analytically and numerically, in [5], leading to the conclusion that their effect is, roughly speaking, negligible and so stability may be studied through the spectral properties of the interaction matrix $\mathbf{A}$. Thus, in agreement with the existing literature [6], we evaluate stability by looking into the maximum real part of the interaction matrix eigenvalues, which we denote $\lambda^*$. The results are presented in Fig. S10 where the leading eigenvalue of the interaction matrix is expressed as a function of the system parameters. As for feasibility, community turns out to be stable over a wide portion of the parameter space as already discussed.

Here, a final note is in order. To be sure, the states with all extinct species are absorbing states of dynamics such as (S1), which means that any observed steady state is only metastable. The times a system like this takes to undergo so strong a fluctuation that drives some species to extinction are so long though that we can ignore this sort of (catastrophic) events here.

# S4 Weak-interaction regime

With "weak-interaction regime" we refer to a situation in which the dynamical contribution of pairwise couplings (the off-diagonal entries of $\mathbf{A}$) is negligible compared to the logistic term (the diagonal terms of $\mathbf{A}$). In other words, the effect of interactions is of a magnitude scale much smaller than that associated with the logistic evolution.

Focusing on the behavior of the system at the stationary state, the right-hand side (S5) may be expressed as

$$1 + \sum_{j=1}^{S} a_{ij}\bar{x}_j = 1 - \frac{\bar{x}_i}{K_i}\left(1 - \sum_{i=1,\, j\neq i}^{S} K_i a_{ij}\frac{\bar{x}_j}{\bar{x}_i}\right), \tag{S7}$$

where we separate the two contributions (diagonal and off-diagonal) of $\mathbf{A}$. Accordingly the "weak-interaction regime" requires

$$\sum_{i=1,\, j\neq i}^{S} K_i a_{ij}\frac{\bar{x}_j}{\bar{x}_i} \ll 1. \tag{S8}$$

Note that, in this regime and assuming a $w\tau_i \ll 1$, (S5) implies $\bar{x}_i \approx K_i$ for all $i = 1, \dots, S$. With this simplification (S8) becomes

$$\sum_{i=1,\, j\neq i}^{S} a_{ij}K_j \ll 1. \tag{S9}$$

But $a_{ij} \sim \mathcal{N}(0, \sigma)$, so

$$\sum_{i=1,\, j\neq i}^{S} a_{ij}K_j \sim \mathcal{N}(0, \Sigma), \qquad \Sigma = \sigma K_{\max}\sqrt{C(S-1)}, \tag{S10}$$

where $K_{\max} = \max_i(K_i)$. Hence, condition (S9) becomes (for $S \gg 1$)

$$\sigma K_{\max}\sqrt{CS} \ll 1. \tag{S11}$$

# S5 A mechanistic explanation of the lognormal mean abundance distribution

Equation (S5) proves that species interactions, embodied in matrix $\mathbf{A}$, shift the average abundances $\bar{x}_j$ so that, even if all carrying capacities were the same ($K_i = K$), the average abundances would split over a wide range of values. Such an effect suggests that there might be interaction matrices that give rise to a lognormal distribution of these average abundances. In this section, we show a way to find matrices with this property for which a feasible and stable community exist. This provides a different mechanism for the appearance of the lognormal mean abundance distribution, putting the burden of explaining its origin in the structure of pairwise species couplings.

For the sake of simplicity, let us assume constant carrying capacities and growth rates, i.e., $a_{ii} = -K^{-1}$ and $\tau_i = \tau$ for all $i = 1, \ldots, S$. From (S5) and denoting $\mathbf{B} \equiv \mathbf{A}^{-1}$, one obtains

$$\bar{x}_i = \gamma \sum_{j=1}^{S} b_{ij}, \qquad \gamma \equiv \frac{w\tau}{2} - 1. \tag{S12}$$

This equation implies that in order for the average abundances $\bar{x}_i$ to follow a lognormal distribution, the sums of the rows of $\mathbf{B}$ must follow such a distribution. We may adopt a mean-field approach here, and postulate that row $i$ of matrix $\mathbf{B}$ has $\kappa_i$ nonzero entries. Then

$$\sum_{j=1}^{S} b_{ij} \sim \mu_{\mathrm{MF}}\kappa_i + \sigma_{\mathrm{MF}}\sqrt{\kappa_i}\eta_i \tag{S13}$$

where $\eta_i \sim \mathcal{N}(0,1)$ is a random Gaussian variable. Now, if we choose $\log\kappa_i \sim \mathcal{N}(\mu_{\mathrm{LN}}, \sigma_{\mathrm{LN}})$ then the left-hand sum is a lognormal random variable (either because $\sigma_{\mathrm{MF}} \ll \mu_{\mathrm{MF}}$ or, if $\mu_{\mathrm{MF}} = 0$, because $\sqrt{\kappa_i}$ is also a lognormal random).

This suggests the following algorithm to obtain an interaction matrix $\mathbf{A}$. For each row $i$:

1. Choose an integer $\kappa_i$ such that $\log\kappa_i \sim \mathcal{N}(\mu_{\mathrm{LN}}, \sigma_{\mathrm{LN}})$.

2. Set $\kappa_i$ random entries of the $i$th row of $\mathbf{B}$ by sampling a distribution $\mathcal{N}(\mu_{\mathrm{MF}}, \sigma_{\mathrm{MF}})$; set the rest to zero.

Finally, to ensure the stability of the community, subtract a positive constant from all the diagonal elements of $\mathbf{B}$.

Figure S11 shows how this algorithm produces interaction matrices able to reproduce all three macroecological laws. Needless to say this is just a proof of concept. Further research is necessary in order to fully characterize the set of interaction matrices that may exhibit a similar behavior.

# S6 Abundance correlation distribution

The Pearson's correlation coefficient between the abundance of species $i$ and $j$ is given by

$$\rho_{ij} = \frac{\mathrm{Cov}(x_i, x_j)}{\sqrt{\mathrm{Var}(x_i)\mathrm{Var}(x_j)}}. \tag{S14}$$

The distribution $\rho_{ij}$ can be computed using a frequentist approximation

$$p(\rho) = \frac{2}{S(S-1)} \sum_{i>j} \delta(\rho - \rho_{ij}), \tag{S15}$$

where $S$ is the species number and the normalization factor $S(S-1)/2$ counts the total number of independent entries of the symmetric matrix $\rho_{ij}$.

Microbial biomes usually contain a large number of species, i.e. $S \sim 10^4$. Simulating *in-silico* communities with such a diversity requires a high computational cost. Specifically, in the analysis of species abundance correlations one has to handle with $S(S-1) \sim 10^8$ Pearson's coefficients.

We aim to reduce the total number of species of each biome by applying an occupancy filter, namely we only keep species present in at least a fraction $o$ of samples ($0 \leq o \leq 1$) termed "occupancy". In Fig. S8, we show the empirical correlation distributions with different occupancy filters. It is possible to see that the same distribution arises for almost all the biomes, regardless of the value of $o$.

In conclusion, we mostly look into high occupancy values, which allows us to reduce the number of species, so that the general computational cost is reduced without blurring the macroecological patterns (in particular, the correlation distribution).

# S7 Environmental fluctuations of shared factors: environmental filtering

Capturing empirical correlations calls for a mechanism to couple the species abundances. In this section, we show that coupling the environmental noise preserves the gamma abundance fluctuation distribution by construction, but it is unlikely to reproduce the experimental correlation distributions.

We consider the Stochastic Logistic Model (SLM) endowed by non-diagonal environmental noise matrix:

$$\dot{x_i} = \frac{x_i}{\tau_i}\left(1 - \frac{x_i}{K_i}\right) + x_i\xi_i, \tag{S16}$$

where $\tau_i$ is the time scale of basal population growth, and $\xi_i$ is a zero-mean, Gaussian, white noise with correlations $\langle \xi_i(t)\xi_j(t')\rangle = w_{ij}\delta(t-t')$. Matrix $\mathbf{W} = (w_{ij})$ accounts for environmental fluctuations, in particular, we sample $w_{ii}$ from a Gaussian distribution with mean and variance given respectively by $\mu_i^{(w)}$ and $\sigma_i^{(w)}$), where $\mu_i^{(w)}$ is the strength of the environmental fluctuations experimented by species $i$, $\sigma_i^{(w)}$ its variability. When $i \neq j$, $w_{ij}$ describes the resource preference of the pair of species $(i, j)$, thus if $w_{ij} > 0$ species have a preference for the same resources/environmental conditions, whereas they have an opposite preference if $w_{ij} < 0$. Such a coupling through environmental noise produces a type of interaction that is referred to in the literature as *environmental filtering*.

The environmental fluctuation matrix $\mathbf{W}$ is the covariance matrix of the Gaussian noise

$$P(\boldsymbol{\xi}) = \frac{1}{\sqrt{2\pi \det \mathbf{W}}} \exp\left\{-\frac{1}{2}\boldsymbol{\xi}^T\mathbf{W}^{-1}\boldsymbol{\xi}\right\}, \tag{S17}$$

thus $\mathbf{W}$ must be a positive definite matrix (i.e. $\boldsymbol{\xi}^T\mathbf{W}\boldsymbol{\xi} > 0$ for all $\boldsymbol{\xi}$).

## S7.1 Environmental filtering preserves the gamma abundance fluctuation distribution by construction

The Langevin dynamics described by (S16) is associated to the Fokker-Planck equation

$$\frac{\partial}{\partial t}P(\mathbf{x}, t) = -\sum_{i=1}^{\infty}\frac{\partial}{\partial x_i}\left[A_i(\mathbf{x})P(\mathbf{x}, t)\right] + \frac{1}{2}\sum_{i,j=1}^{\infty}\frac{\partial^2}{\partial x_i \partial x_j}\left[w_{ij}x_ix_jP(\mathbf{x}, t)\right], \tag{S18}$$

where

$$A_i(\mathbf{x}) = \frac{x_i}{\tau_i}\left(1 - \frac{x_i}{K_i}\right). \tag{S19}$$

Equation (S18) allows us to obtain the abundance fluctuation distribution of species $k$, i.e. the marginal of $P(\mathbf{x}, t)$. To do so we marginalize (S18) with respect to an arbitrary species $k$ as

$$\int_{\mathbb{R}_+^{N-1}} d^{N-1}\mathbf{x}_{\hat{k}} P(\mathbf{x}, t) = \bar{P}_k(x_k, t), \tag{S20}$$

where $\mathbf{x}_{\hat{k}} = (x_1, x_2, \dots, x_{k-1}, x_{k+1}, \dots, x_N)$ is a vector in which the abundance of species $k$ is absent. The drift term when $i = k$ marginalizes to

$$\frac{\partial}{\partial x_k} \int_{\mathbb{R}_+^{N-1}} d^{N-1}\mathbf{x}_{\hat{k}} \left[A_k(\mathbf{x}) P(\mathbf{x}, t)\right] = \frac{\partial}{\partial x_k} \frac{x_k}{\tau_k}\left[1 - \frac{x_k}{K_k}\right] \int_{\mathbb{R}_+^{N-1}} d^{N-1}\mathbf{x}_{\hat{k}} P(\mathbf{x}, t) = \frac{\partial}{\partial x_k} \frac{x_k}{\tau_k}\left[1 - \frac{x_k}{K_k}\right] \bar{P}_k(x_k, t), \tag{S21}$$

whereas when $i \neq k$ it vanishes because of the boundary conditions on $P(\mathbf{x}, t)$,

$$\int_{\mathbb{R}_+^{N-2}} d^{N-2}\mathbf{x}_{\hat{k}\hat{i}} \int_0^\infty dx_i \frac{\partial}{\partial x_i}\left[A_i(\mathbf{x}) P(\mathbf{x}, t)\right] = \int_{\mathbb{R}_+^{N-2}} d^{N-2}\mathbf{x}_{\hat{k}\hat{i}} \left[A_i(\mathbf{x}) P(\mathbf{x}, t)\right]\Big|_{x_i=0}^{\infty} = 0 \tag{S22}$$

The diffusion term of (S18) is split into four contributions: (i) diagonal term with $i = j = k$, (ii) diagonal terms with $i = j \neq k$, (iii) off-diagonal terms of the form $k \neq i \neq j \neq k$ and (iv) off-diagonal terms with $j = k$ (identical to $i = k$). The first contribution is given by

$$\frac{\partial^2}{\partial x_k^2} \int_{\mathbb{R}_+^{N-2}} d^{N-1}\mathbf{x}_{\hat{k}}\, x_k^2 P(\mathbf{x_k}, t) = \frac{\partial^2}{\partial x_k^2}\left[x_k^2 \bar{P}_k(x_k, t)\right], \tag{S23}$$

whereas the rest of the contributions are null

$$\int_{\mathbb{R}_+^{N-2}} d^{N-2}\mathbf{x}_{\hat{k}\hat{i}} \int_0^\infty dx_i w_{ii} \frac{\partial^2}{\partial x_i^2}\left[x_i^2 P(\mathbf{x}, t)\right] = \int_{\mathbb{R}_+^{N-2}} d^{N-2}\mathbf{x}_{\hat{k}\hat{i}} w_{ii} \frac{\partial}{\partial x_i}\left[x_i^2 P(\mathbf{x}, t)\right]\Big|_{x_i=0}^{\infty} = 0 \tag{S24}$$

$$\int_{\mathbb{R}_+^{N-3}} d^{N-3}\mathbf{x}_{\hat{k}\hat{i}\hat{j}} \int_{\mathbb{R}_+^2} dx_i dx_j w_{ij} \frac{\partial}{\partial x_i \partial x_j} x_i x_j P(\mathbf{x}, t) = \int_{\mathbb{R}_+^{N-3}} d^{N-3}\mathbf{x}_{\hat{k}\hat{i}\hat{j}} \Big[x_i x_j P(\mathbf{x}, t)\Big]\Big|_{x_i=0}^{\infty} = 0 \tag{S25}$$

$$\frac{\partial}{\partial x_k} x_k \int_{\mathbb{R}_+^{N-2}} d^{N-2}\mathbf{x}_{\hat{k}\hat{i}} \int_0^\infty dx_i w_{ik} \frac{\partial}{\partial x_i} x_i P(\mathbf{x}, t) = \frac{\partial}{\partial x_k} x_k \int_{\mathbb{R}_+^{N-2}} d^{N-2}\mathbf{x}_{\hat{k}\hat{i}} w_{ik} \left[x_i P(\mathbf{x}, t)\right]\Big|_{x_i=0}^{\infty} = 0. \tag{S26}$$

Thus, the marginalized expression of (S18) is given by

$$\frac{\partial}{\partial t}\bar{P}_k(x_k, t) = -\frac{\partial}{\partial x_k}\left\{\frac{x_k}{\tau_k}\left[1 - \frac{x_k}{K_k}\right]\bar{P}_k(x_k, t)\right\} + \frac{w_{kk}}{2}\frac{\partial^2}{\partial x_k^2}\left[x_k^2 \bar{P}_k(x_k, t)\right]. \tag{S27}$$

The stationary solution of (S27), i.e. the abundance fluctuation distribution, can be computed by setting the left-hand side to zero:

$$\frac{2}{w_{kk}} \frac{x_k}{\tau_k}\left[1 - \frac{x_k}{K_k}\right] \bar{P}_k^{\mathrm{st}}(x_k) = \frac{d}{dx_k}\left[x_k^2 \bar{P}_k^{\mathrm{st}}(x_k)\right]. \tag{S28}$$

Solving by separation of variables we obtain the expression for the abundance fluctuation distribution of species $i$

$$\bar{P}_i^{\mathrm{st}}(x_i) = \frac{1}{\Gamma\left(\frac{2}{w_{ii}\tau_i} - 1\right)} \left(\frac{2}{K_i w_{ii} \tau_i}\right)^{\frac{2}{w_{ii}\tau_i} - 1} \exp\left(-\frac{2}{K_i w_{ii}\tau_i} x_i\right) x_i^{w_{ii}\tau_i}, \tag{S29}$$

where $w_{ii}\tau_i = \sigma_i^{(w)}$ highlights that the gamma abundance fluctuation distribution only depends on the diagonal terms of environmental fluctuation matrix $\mathbf{W}$. This proves that the gamma abundance fluctuation distribution is held by construction in model (S16).

## S7.2 Random environmental filtering matrix mostly produces positive correlations

The environmental filtering matrix $\mathbf{W} = (w_{ij})$ introduces correlations by coupling species abundances based on their similar or opposite response to environmental changes. For example, if two species share a similar preference for low pH with this increasing during an environmental fluctuation, their response will be similar causing positive correlations.

Empirical correlation distributions display a significant fraction of negative correlations, but since $\mathbf{W}$ is a covariance matrix, it must be positive definite, something which limits its ability to generate negative correlations. In this section, we provide a evidence supporting this.

For this purpose, we use a random environmental matrix and sweep a wide range of the parameter space. For every parameter configuration, we run the dynamics of (S16) and compute the stationary abundance correlation distribution.

In order to produce a positive-definite, symmetric, random matrix $\mathbf{W}$ we factor it as $\mathbf{W} = \mathbf{U}^T\mathbf{\Lambda}\mathbf{U}$, where $\mathbf{U}$ is an $S \times S$ orthogonal matrix ($\mathbf{U}\mathbf{U}^T = \mathbf{U}^T\mathbf{U} = \mathbf{I}$), and $\mathbf{\Lambda}$ is an $S \times S$ diagonal square matrix that contains the eigenvalues of $\mathbf{W}$. In order for this matrix to be positive definite we need that $\lambda_i > 0$ for $i = 1, \ldots, S$. On the one hand, the orthogonal matrix must be randomly sampled from a Haar distribution, which is the only uniform distribution on the orthogonal group $O(S)$. On the other hand, we have explored the dependence with different probability distributions for $\lambda_i$, to maintain the positive-definiteness constraint their support must belong to $\mathbb{R}_+$. In particular Fig. S12 illustrates the results for a beta, a uniform, and a lognormal distributions. In all cases we can see that negative correlations drop very quickly, whereas positive ones can be arbitrarily large.

## S7.3 Bayesian sampling of environmental filtering matrices

According to the exploratory search of the previous section it appears very difficult to generate negative correlations through a noise matrix $\mathbf{W}$. But perhaps the task requires a finer tuning of this matrix. In order to test whether a more structured matrix $\mathbf{W}$ can reproduce the empirical abundance correlation distribution we have carried out a Monte Carlo Markov Chain (MCMC) simulation similar to the one we developed in the main text for the species interaction matrix $\mathbf{A}$, but this time exploring $\mathbf{W}$.

Thus, we sample matrices $\mathbf{W}$ by applying a Metropolis-Hastings factor algorithm [1] on the posterior distribution $P(\mathbf{W}|\rho)$. In order to preserve the positive-definiteness of $\mathbf{W}$ we resort to the orthogonal decomposition $\mathbf{W} = \mathbf{U}^T\mathbf{\Lambda}\mathbf{U}$ and proceed as follows. At each Monte Carlo step $n$ we perform a transformation

$$\mathbf{U}^{(n+1)} = \mathbf{R}\mathbf{Q}\mathbf{R}^T\mathbf{U}^{(n)}\mathbf{R}^T\mathbf{Q}^T\mathbf{R}, \qquad \text{(S30)}$$

where $\mathbf{R}$ is a random matrix of the group $SO(S)$ and $\mathbf{Q}$ is either the identity matrix with a random element of the diagonal set to $-1$, or the box diagonal matrix

$$\mathbf{Q} = \begin{pmatrix} \mathbf{P}(\theta) & \mathbf{0} \\ \mathbf{0} & \mathbf{I}_{S-2} \end{pmatrix}, \qquad \mathbf{P}(\theta) = \begin{pmatrix} \cos\theta & -\sin\theta \\ \sin\theta & \cos\theta \end{pmatrix}, \qquad \theta \sim \mathcal{U}[-0.01\pi, 0.01\pi]. \qquad \text{(S31)}$$

Alternatively, we change a random element of the diagonal of $\mathbf{\Lambda}^{(n)}$ as

$$\lambda_i^{(n+1)} = \Lambda_i^{(n)} + \eta, \qquad \eta \sim \mathcal{U}\left[-0.01\lambda_i^{(n)}, 0.01\lambda_i^{(n)}\right], \qquad \text{(S32)}$$

with the proviso that $\lambda_i^{(n+1)}$ must remain positive.

Finally, the environmental filter matrix to run the next dynamics is obtained as $\mathbf{W}^{(n+1)} = \mathbf{U}^{(n+1)T}\mathbf{\Lambda}^{(n+1)}\mathbf{U}^{(n+1)}$ and the algorithm proceeds as in the Bayesian approach for $\mathbf{A}$ explained in the "Materials and Methods" of the main text.

Figure S19 shows the distance from the logarithm of the generated correlation distribution to the empirical one, in a typical run of the MCMC. For comparison, we have included the graph corresponding to a MCMC performed on the interaction matrix $\mathbf{A}$. The results clearly show that this method is incapable of finding a region of the space of physical noise matrices where correlations are correctly reproduced.

# S8 Search for statistical patterns in the interactions

We have investigated several features in search for statistical patterns in the interaction matrices generated through Monte Carlo simulations, with the aim of characterizing the ensemble. However, none of them provides a clear distinction with respect to a set of random matrices. The test we have made are the following (in all cases, except the last one, averages are taken over 200 sample matrices):

**Distribution of ecological interactions:** We have calculated the proportion of interactions within different ecological categories. The results, illustrated in the radar plot of Figure S20(a), indicate that the distribution of interactions is consistent across both types of matrices.

**Degree distribution of the interaction network:** We have analyzed the incoming and outgoing degree distributions of the interaction network and presented the results in Figure S20(b). As shown in this figure, there is no noticeable difference in the degree distributions between the two types of matrices.

**Counting loops in the interaction network:** We have quantified the number of closed paths of various lengths in both sets of matrices. This involved converting non-zero entries in matrix $\mathbf{A}$ to ones and computing $\mathrm{tr}(\mathbf{A}^n)$ for different lengths $n$. Figure S20(c) demonstrates that there is no distinction in the number of closed paths between matrices generated through Monte Carlo simulations and random matrices.

**Spectral distribution:** Figure S20(d) compares the distribution of complex eigenvalues for two sets of ten matrices each, obtained through Monte Carlo simulations (left panel) and randomly generated matrices (right panel). There are no discernible features that differentiate the two sets.

# S9 Supplementary Figures and Tables

| Mode | Mean | Variance | Skewness | Biome |
|---|---|---|---|---|
| $0.0529314$ | $0.030$ | $0.015$ | $1.24$ | Sludge |
| $0.0645295$ | $0.061$ | $0.027$ | $1.23$ | Gut1 |
| $-0.0503573$ | $0.044$ | $0.035$ | $1.30$ | Soil |
| $-0.0723794$ | $0.015$ | $0.023$ | $1.31$ | Lake |
| $-0.186763$ | $0.018$ | $0.072$ | $0.95$ | Oral1 |
| $0.0223393$ | $0.032$ | $0.042$ | $0.91$ | Seawater |
| $0.00485029$ | $0.026$ | $0.073$ | $0.54$ | Glacier |
| $-0.0181499$ | $0.041$ | $0.032$ | $0.99$ | River |
| $-0.0958909$ | $0.035$ | $0.038$ | $1.39$ | Gut2 |

Table S1: First three cumulants of the Pearson's abundance-correlation distribution for different biomes. Mean ($m$), variance ($s^2$), and skewness ($b$) are obtained from: $m = n^{-1} \sum_i x_i$, $s^2 = (n-1)^{-1} \sum_i (x_i - m)^2$, and $b = s^{-3} n^{-1} \sum_i (x_i - m)^3$. Values of $b > 1$ are taken to indicate a strong (positive) skewness, whereas those $0.5 < b < 1$ indicate weak (positive) skewness.

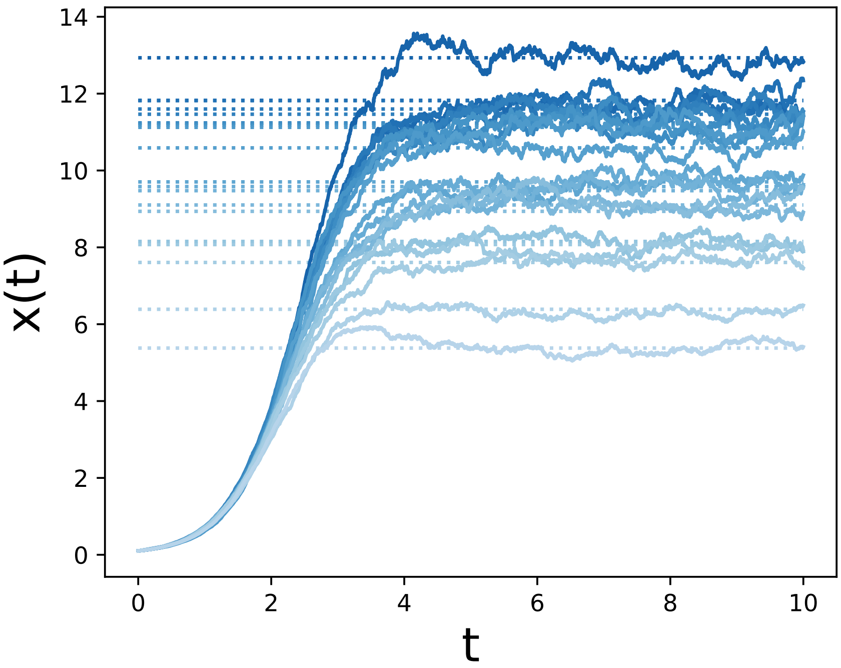


Figure S1: **Stochastic Lotka-Volterra dynamics**. Numerical solution of the Stochastic Lotka-Volterra equation (S1) obtained by means of the *Euler-Maruyama* method. The plot describes the population dynamics of $S = 20$ species with the same carrying capacity $K_i = K = 10$ and intrinsic growth time $\tau_i = \tau = 0.5$, $i = 1, ..., S$, in the case of non-correlated noise $w_{ij} = w\delta_{ij}$ with $w = 0.1$. Lotka-Volterra constants $a_{ij}$ are sampled from a normal distribution $\mathcal{N}(0, 0.005)$. Overall, the model describes stochastic fluctuations around mean abundances shifted by interactions according to (S5) of the main text.

# References


[1] R. Toral, P. Colet - Stochastic Numerical Methods *Wiley-VCH, Weingheim, Germany*, 96, 373, (2014)

[2] J. Grilli - Macroecological laws describe variation and diversity in microbial communities *Nat. Comm*, 11, 1-11, (2020)

[3] P. Rohr, S. Saavedra, J. Bascompte - On the structural stability of mutualistic systems *Science*, 345, 1253497 (2014)

[4] S. Saavedra, R.P. Rohr, J.M. Olesen, J. Bascompte - Nested species interactions promote feasibility over stability during the assembly of a pollinator community *Ecol. evolution*, 6, 997–1007 (2016)

[5] T. Gibbs, J. Grilli, T. Rogers, S. Allesina, - Effect of population abundances on the stability of large random ecosystems *Physical Review E*, 98, 022410 (2018)

[6] S. Allesina, S. Tang - Stability criteria for complex ecosystems *Nature*, 483, 205 (2012)

[7] A.L. Mitchell *et al.* - Ebi metagenomics in 2017: enriching the analysis of microbial communities, from sequence reads to207 assemblies *Nucleic Acids Res.*, (2018)

[8] S. Kéfi *et al.* - Advancing our understanding of ecological stability *Ecology Letters, 22, 9, 1349–1356*, (2019)

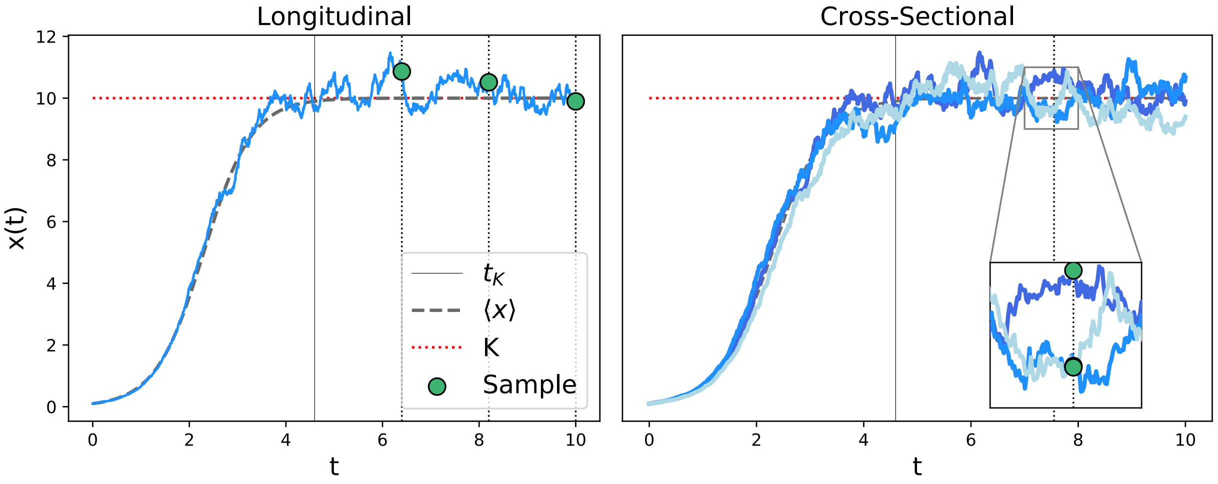


Figure S2: The left plot illustrates longitudinal samples (green bullets), representing abundances from the same realization but at different times. The right plot depicts cross-sectional samples (green bullets), indicating abundances selected from different realizations. In both cases, sampling occurs once the stationary state is achieved, *i.e.*, for times greater than $t^{(st)}$. This time denotes when the average population $\bar{x}$ approximately matches the stationary state $\bar{x}^{(st)}$ (refer to Eq. (2) in the main text), allowing for a 1% error. Averages are calculated over fluctuations.

[9] L. Descheemaeker *et al.* - Stochastic logistic models reproduce experimental time series of microbial communities *eLife 2020;9:e55650*, (2020)

[10] A. George *et al.* - Universal abundance fluctuations across microbial communities, tropical forests, and urban populations *PNAS 120:e2215832120*, (2023)

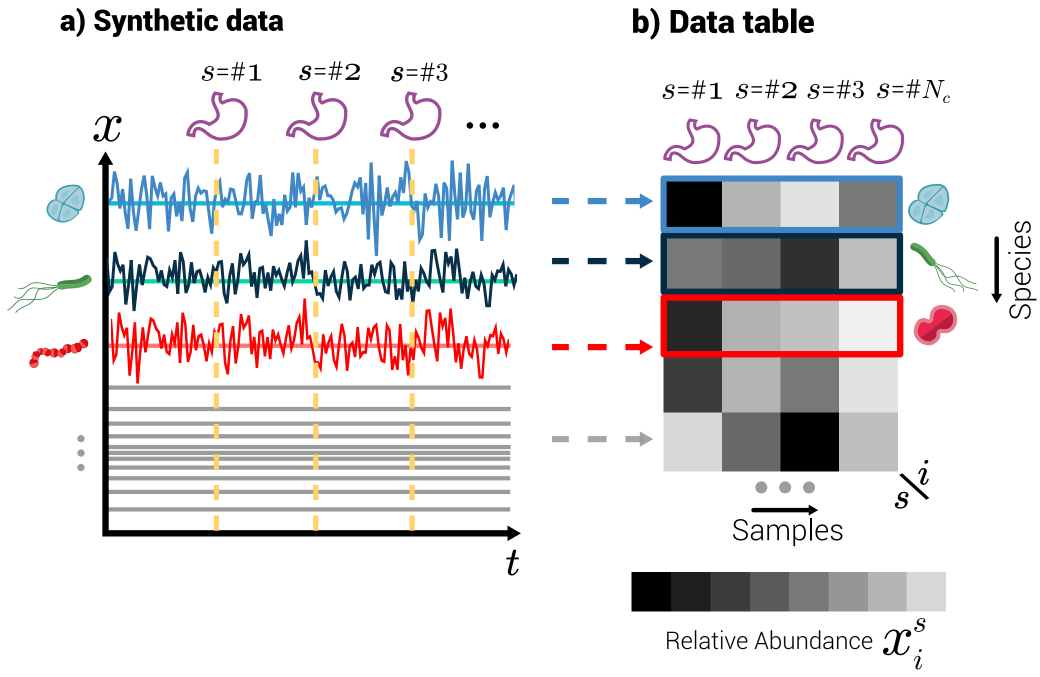


Figure S3: **Species-samples table of abundances a)** Stochastic fluctuations of species abundances at the stationary state of (S1). Longitudinal samples are selected at times represented by yellow dashed lines. **b)** The species abundances obtained in different samples may be arranged in a matrix, with rows (columns) given by the species (samples). Entry $(i, s)$ of the matrix contains the abundance of the species $i$ in sample $s$.

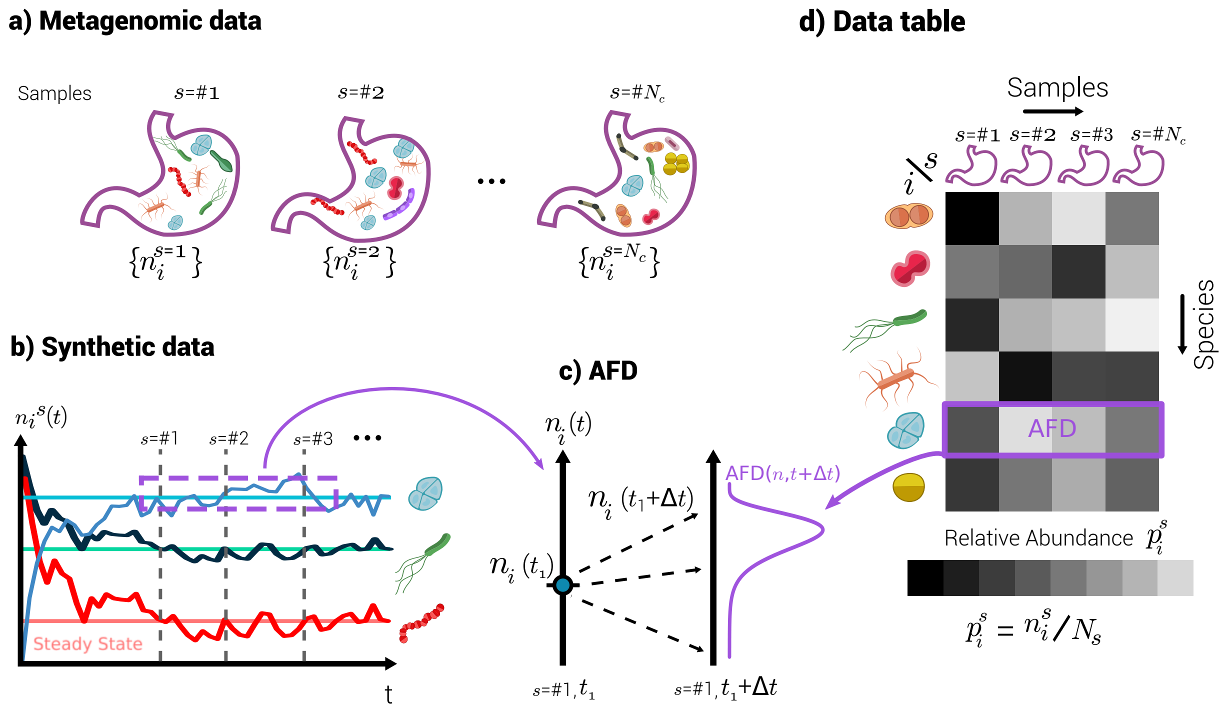


Figure S4: **Comparison between empirical and synthetic data**. **a)** Experimental data are collected via metagenomic analysis, so they refer to different samples of genetic material selected directly in its natural environment. For instance, in the case of a gut biome, one may observe the gut flora from one patient over time, or at a fixed time for different patients. In general, the dataset of a biome $\mathcal{B}$ consists of a set of counts $\{n_i^s\} = \{n_1^s, n_2^s, \dots\}$, where $n_i^s$ is the total number of occurrences of species $i = 1$ on sample $s$. **b)** *In silico* biomes can be generated through the corresponding population dynamics. Once the system has reached the stationary state the joint probability distribution, $p(n_1, \dots, n_S)$, stops evolving, so the probability of finding $n_i$ counts of species $i$ in a sample remains constant. **c)** The abundance fluctuation distribution (AFD) describes the distribution of abundance across samples. **d)** Sketch of a typical abundance data table. For each biome the information about the abundances of species in each sample (metagenomic or *in silico* data) can be arranged in a table (in wide format), with species along the rows and communities along the columns.

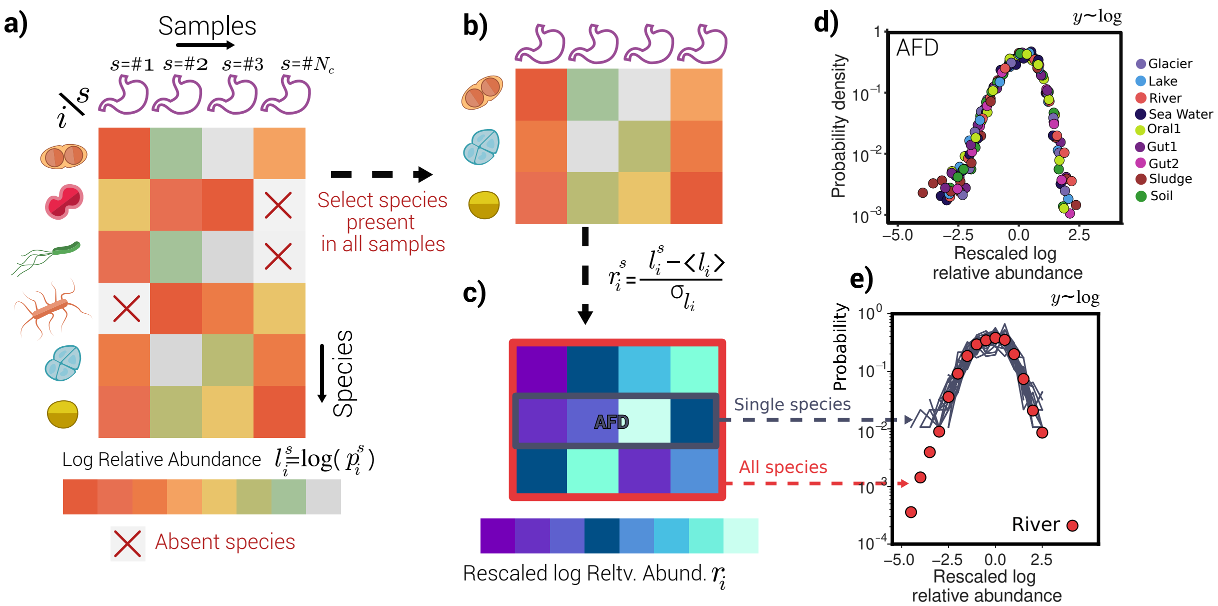


Figure S5: **Abundance fluctuation distribution**. **a)** Sketch of a typical (log) abundance data table. **b)** Data cleaning of species that are not present in all samples, i.e., have occurrence $o_i = 1$. **c)** Standard normalization of species abundance fluctuation distribution (AFD) to set their mean values to 0 and variances to 1 (z-score). **d)** Abundance Fluctuation Distribution for a wide variety of biomes. **e)** The tangle of grey lines is the result of the superposition of the plots of the distribution of the single species, while the coloured dots are the result of grouping the distributions of all the species into a single one.

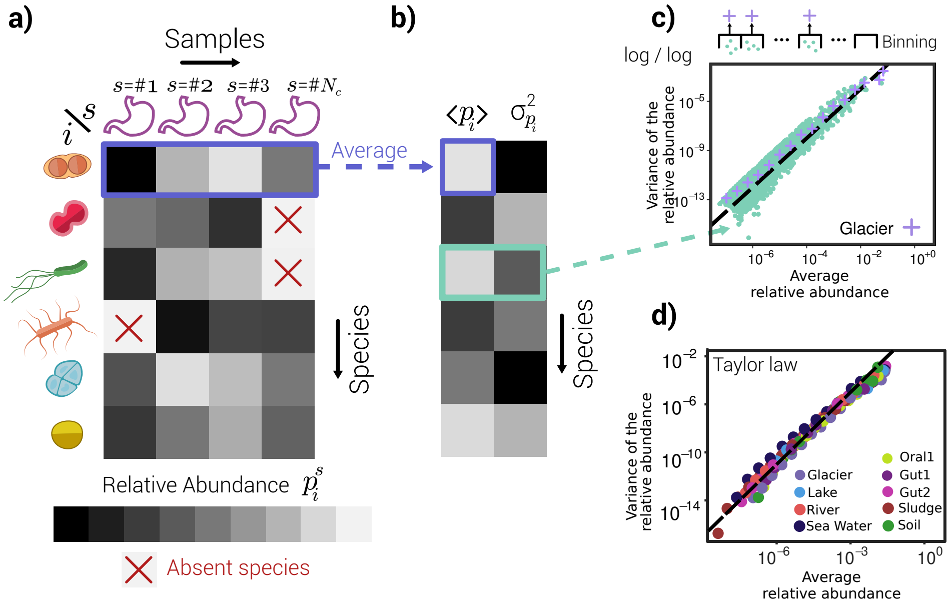


Figure S6: **Data Analysis: Taylor's Law.** **a)** Sketch of a typical abundance data table. **b)** Mean and standard deviation of the abundance across samples. Multiplying by the occupancy is the correct way to include in the calculation the zero abundances of the species in the samples. **c)** The mean and the variance of the abundance across samples are not independent over species, but they hold a power law relationship known as the Taylor Law. Greenish-blue dots correspond to single species, whereas violet crosses correspond to the binning average across species. **d)** Taylor's law is maintained for a wide diversity of biomes.

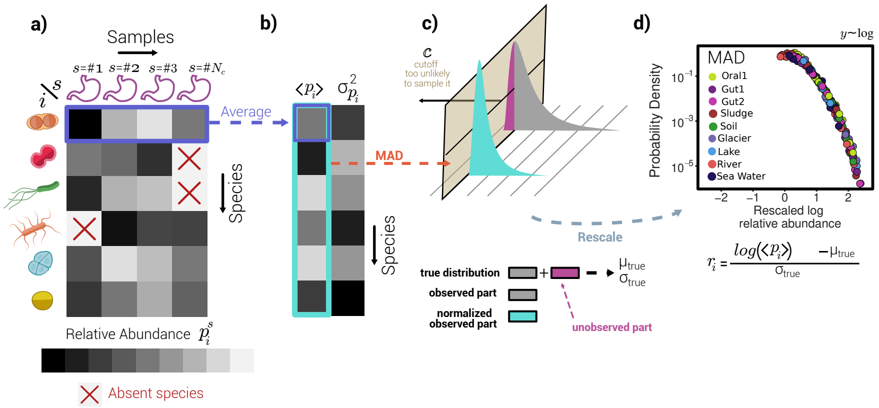


Figure S7: **Data Analysis: Mean Abundance Distribution**. **a)** Sketch of a typical abundance data table. **b)** Mean and standard deviation of the abundance across samples. Multiplying by the occupancy is the correct way to include in the calculation the zero abundances of the species in the samples. **c)** Rare species, i.e. those whose abundance are bellow a threshold ($x_i < c$), are very unlikely to be detected. Thus we observe only the right part of the true distribution ($\rho_{\mathrm{true}}(\bar{x})$ , grey part), whose normalization is given by the blue distribution ($\rho_b(\bar{x})$). **d)** Mean abundance distribution (MAD) for a wide range of biomes.

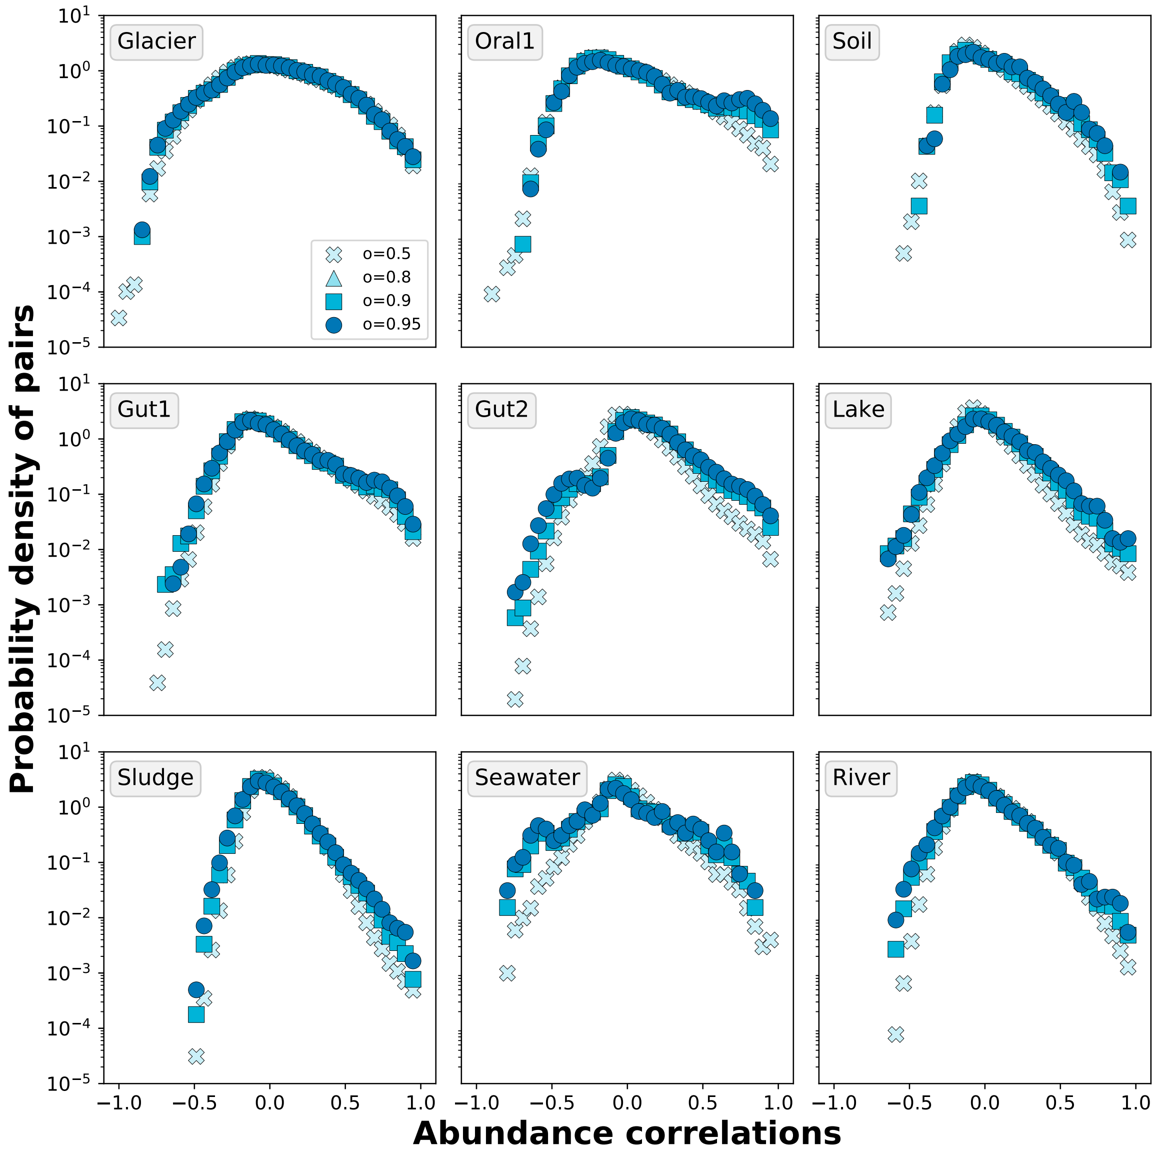


Figure S8: **Empirical correlation distributions for different occupancy filters**. Abundance correlation distributions for nine real biome data selected from the platform selected from the *EBI metagenomics* platform [7]. For each biome we present the distribution related to different occupancy values $o$, expressing the minimum fraction of samples where a given species is present.

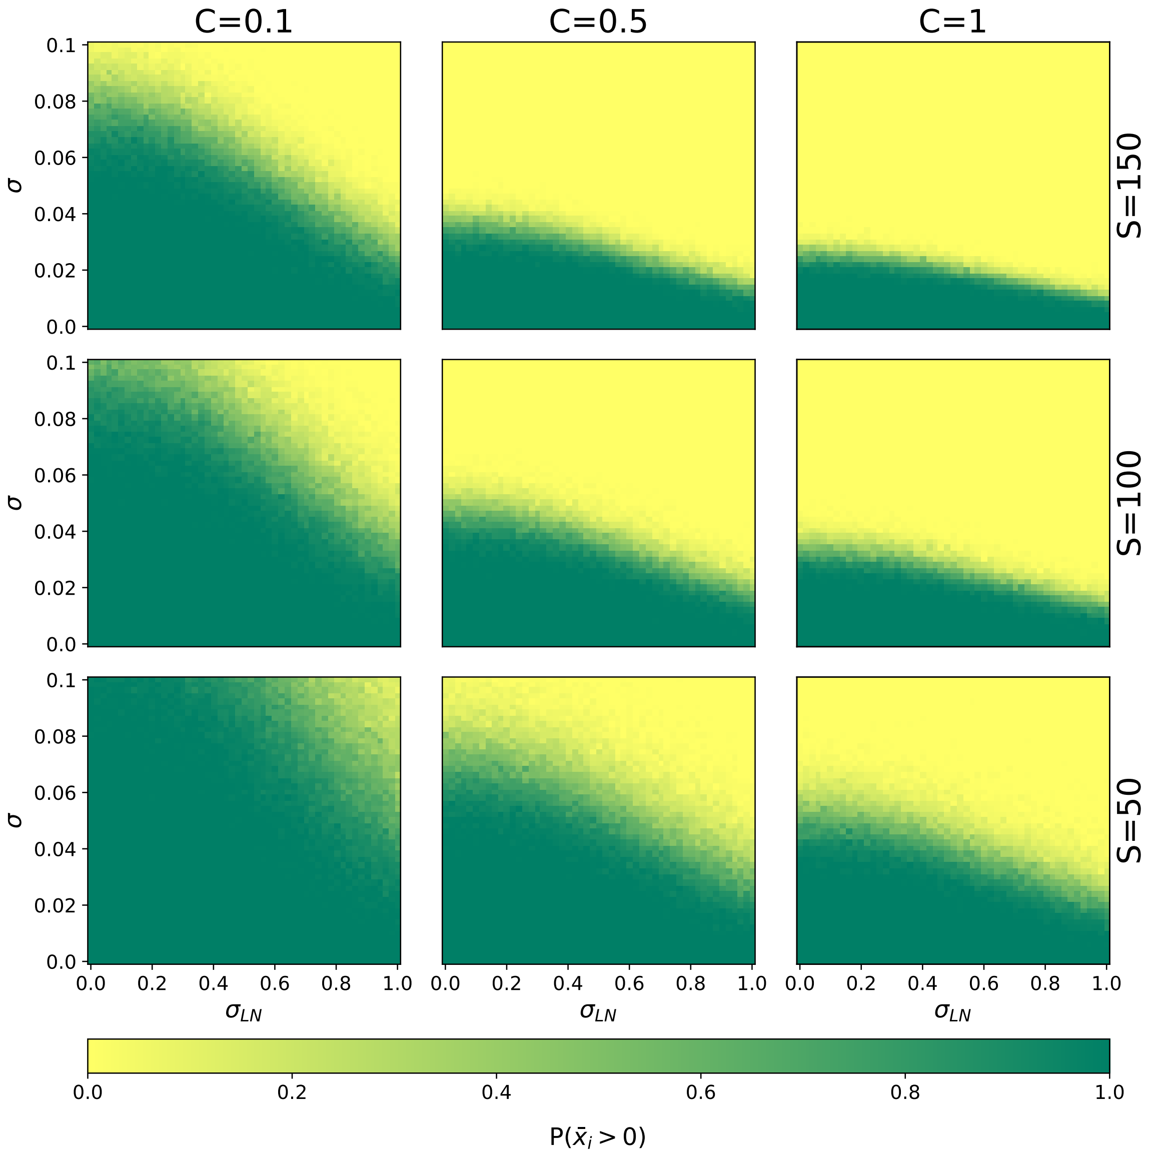


Figure S9: **Feasibility diagram**. Probability that a community has a feasible steady state ($\bar{x}_i > 0$ for all $i = 1, ..., S$) as a function of the sampling parameters of the interaction matrices $\mathbf{A}$. Different panels display results for different combinations of the connectance $C$ and the number of species $S$. For each choice of $\sigma$ and $\sigma_{LN}$, we generate a sample of 100 interaction matrices $\mathbf{A}$ with diagonal elements $a_{ii} = -1/K_i$ ($K_i \sim \mathcal{N}(\mu_{LN}, \sigma_{\mathrm{LN}})$) and a fraction $C$ of nonzero off-diagonal elements $a_{ij} \sim \mathcal{N}(0, \sigma)$. For each interaction matrix, we calculate the corresponding stationary abundances from (S6) (neglecting the noise term) and evaluate the fraction of feasible communities out of them. This fraction is represented using a color code.

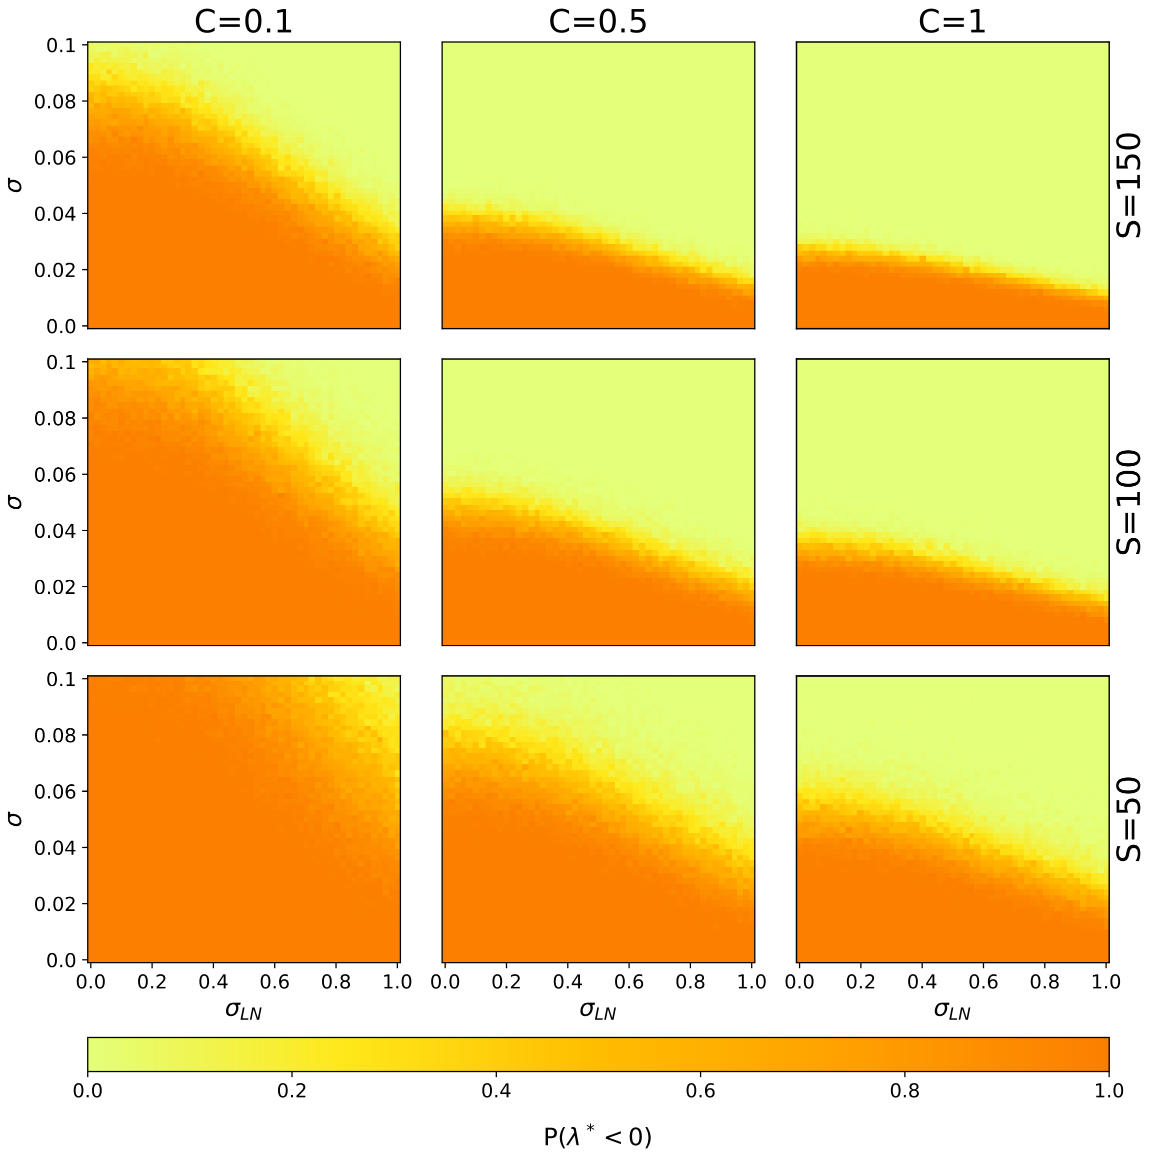


Figure S10: **Stability diagram**. Probability that the system has an asymptotically stable stationary state (i.e. the maximum real part eigenvalue of the interaction matrix is negative). Different panels display results for different combinations of the connectance $C$ and the number of species $S$. For each choice of $\sigma$ and $\sigma_{LN}$, we generate a sample of 100 interaction matrices $\mathbf{A}$ with diagonal elements $a_{ii} = -1/K_i$ ($K_i \sim \mathcal{N}(\mu_{LN}, \sigma_{\mathrm{LN}})$) and a fraction $C$ of nonzero off-diagonal elements $a_{ij} \sim \mathcal{N}(0, \sigma)$. Then we calculate the probability that the system is stable for those parameters as the fraction matrices all whose eigenvalues have no positive real part. This fraction is represented using a color code.

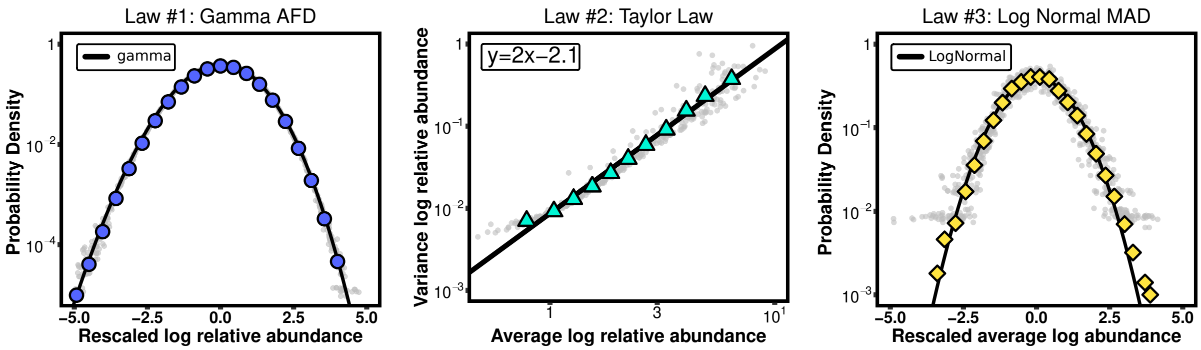


Figure S11: **Simulated Macroecological Laws by properly engineering species interactions**. The emergence of a gamma abundance fluctuation distribution (AFD) seems to be independent of the interactions and a direct consequence of the multiplicative noise; however, the emergence of both Taylor's law and the lognormal mean abundance distribution (MAD) is a highly nontrivial result because these two macroscopic patterns can be engineered in different ways. Here, we show that a lognormal mean abundance distribution can emerge by a suitable choice of the interaction matrix while keeping the carrying capacities uniform for all species (see Sec. S5). Also, panel **(b)** shows that this choice does not spoil Taylor's law. The grey points in the background of the three panels are the results of a sample of $N = 50$ interactions networks $\mathbf{A}$, whereas the coloured points are the averages across networks. Parameters: $\mu_{\mathrm{G}} = 0.5$, $\sigma_{\mathrm{G}} = 0.6$, $\mu_{\mathrm{MF}} = -0.5$, $\sigma_{\mathrm{MF}} = 0.3$, $\sigma^{(w)} = 0.4$, $S = 500$, $\tau = 0.1$, $K = 1$.

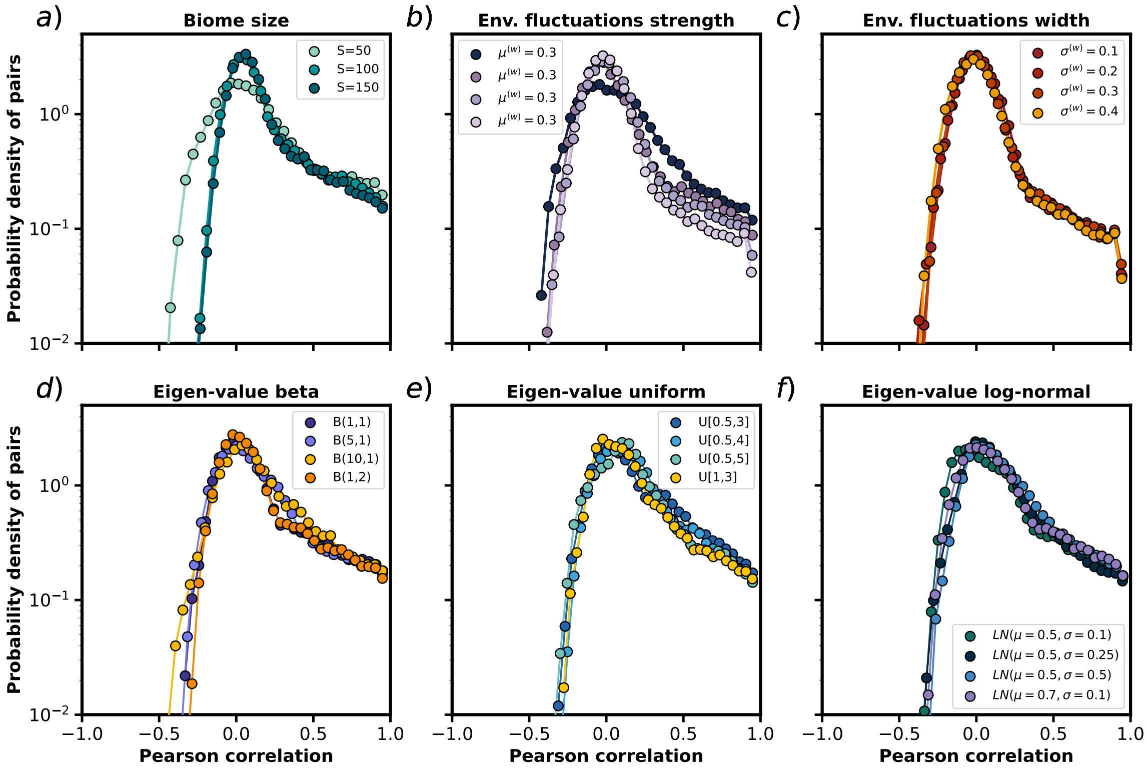


Figure S12: **Environmental filtering mostly produces positive correlations**. Panels portray Pearson's abundance correlation distributions (see (S14)) produced by environmental filtering alone (matrix $\mathbf{W}$). In panels **(a)–(c)** we study the results as for different values of one parameter of the model: biome size $S$, environmental fluctuations strength $\mu^{(w)}$, and standard deviation of environmental fluctuations $\sigma^{(w)}$. In panels **(d)–(f)** we study the influence of the eigenvalue distribution of the environmental filtering matrix $\mathbf{W}$. Our results show that, regardless of the choice of parameters or the distribution of eigenvalues, the positive definiteness of matrix $\mathbf{W}$ results in a severe lack of negative correlations. The correlations distributions are strongly asymmetric, showing a peak at zero.

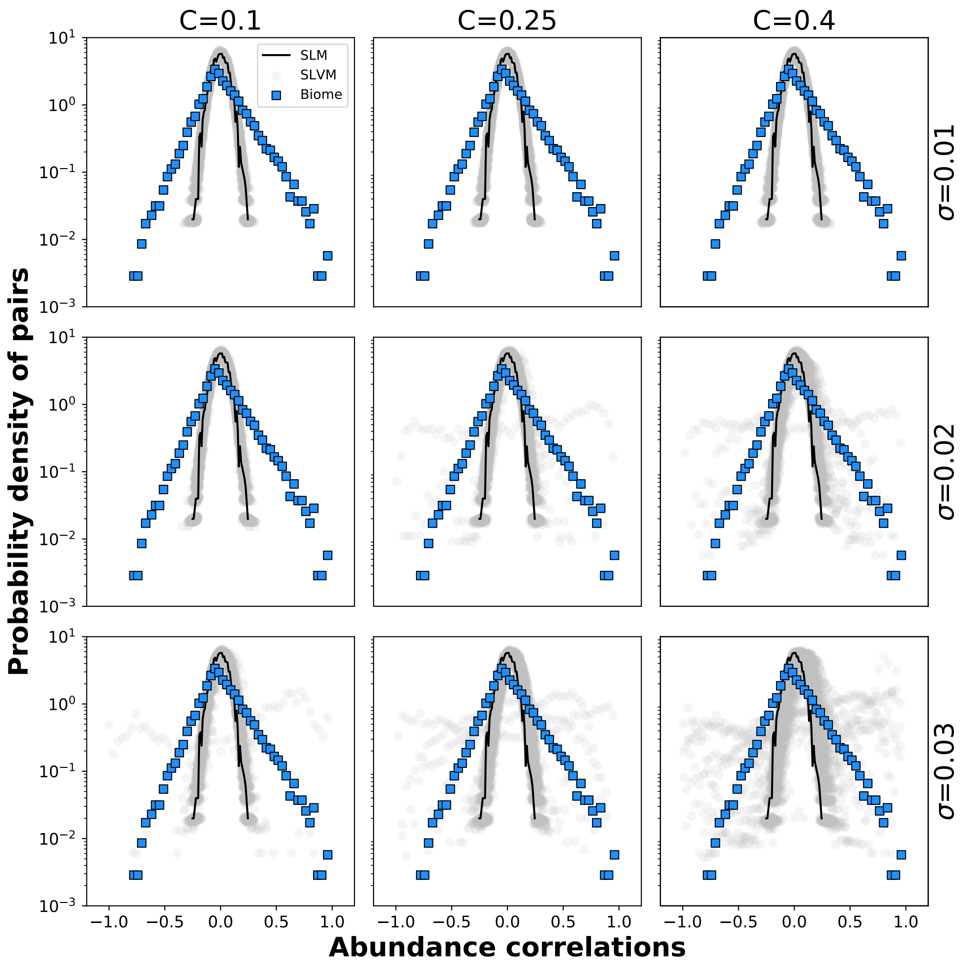


Figure S13: **Abundance correlation distributions as a function of some interaction parameters**. Blue squares portray the empirical distribution obtained for the *Seawater* biome with occupancy $o = 0.5$ (i.e. keeping only the species appearing in at least the $50\%$ of the environmental samples). Black solid lines depict the distribution obtained with the SLM, while grey dots are the results produced by the SLVM. Here, interaction constants have been sampled from a normal distribution $\mathcal{N}(0, \sigma)$, with $\sigma = 0.01, 0.02, 0.03$ (corresponding to the different rows of the plot grid). The connectance has been set to $C = 0.1, 0.25, 0.4$ and varies across columns of the grid. In all cases the number of species is equal to $S = 100$ and the carrying capacities have been sampled from a lognormal distribution with $\mu_{\mathrm{LN}} = 0.1$ and $\sigma_{\mathrm{LN}} = 0.5$. Correlations occur among abundances resulting from a dynamics run with $\tau = 0.1$ and $w = 0.01$. We can see that, at odds with the results from the SLM, the distributions obtained with the SLVM approximately cover the whole range of Pearson coefficients $-1 \leq \rho_{ij} \leq 1$, suggesting the suitability of the SLVM to fit the empirical patterns. Similar results are obtained for different values of the parameters $S$, $w$, $\mu$, $\mu_{\mathrm{LN}}$, and $\sigma_{\mathrm{LN}}$.

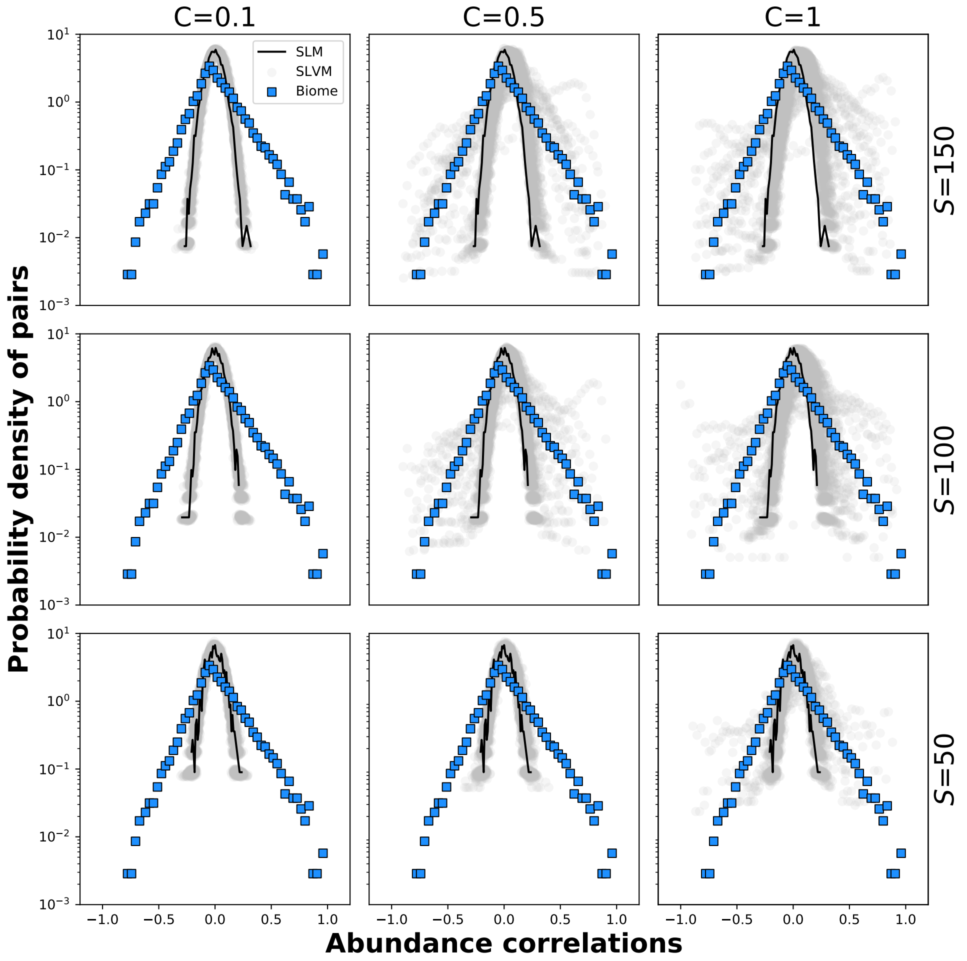


Figure S14: **Abundance correlation distribution as a function of some interaction parameters**. Blue squares portray the empirical distribution obtained for the *Seawater* biome with occupancy $o = 0.5$ (i.e. keeping only the species appearing in at least the $50\%$ of the environmental samples). Black solid lines depict the distribution obtained with the SLM, while grey dots are the results produced by the SLVM. Here, interaction constants have been sampled from a normal distribution $\mathcal{N}(0, 0.01)$. The connectance has been set to $C = 0.1$, $0.25$, $0.4$ and varies across columns of the grid. The number of species is equal to $S = 50$, $100$, $150$ and varies across rows. The carrying capacities have been sampled from a lognormal distribution with $\mu_{\text{LN}} = 0.1$ and $\sigma_{\text{LN}} = 0.5$. Correlations occur among abundances resulting from a dynamics run with $\tau = 0.1$ and $w = 0.01$. We can see that, at odds with the results from the SLM, the distributions obtained with the SLVM approximately cover the whole range of Pearson coefficients $-1 \leq \rho_{ij} \leq 1$, suggesting the suitability of the SLVM to fit this empirical patterns. Similar results are obtained for different values of the parameters $\sigma$, $w$, $\mu$, $\mu_{\text{LN}}$, and $\sigma_{\text{LN}}$.

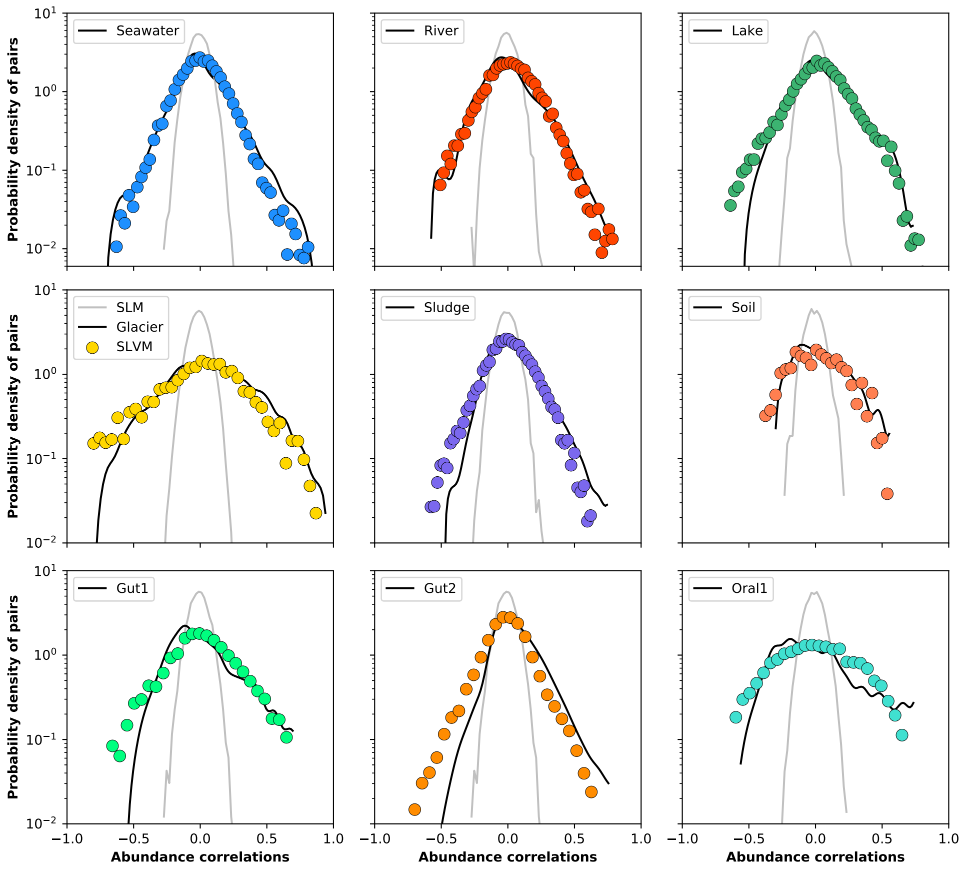


Figure S15: **MCMC correlation distributions** Abundance correlation distributions for both empirical and synthetic microbial communities. Each plot corresponds to a real biome, and its empirical distribution is represented by a black solid line. Colored bullets represent Pearson's correlation distribution of abundances calculated using (S1) with Lotka-Volterra interactions $\{a_{ij}\}_{i\neq j}$ obtained through the algorithm described in the 'Material and Methods' section of the main text. The grey solid lines portray the distributions resulting from the SLM [2], i.e. without interactions ($\{a_{ij}\}_{i\neq j} = 0$). The model struggles to fit the skewed distributions exhibited by some biomes, like *Oral1*, which suggests that, as discussed in the main text, those cases might require the presence of both, interactions and an environmental filtering.

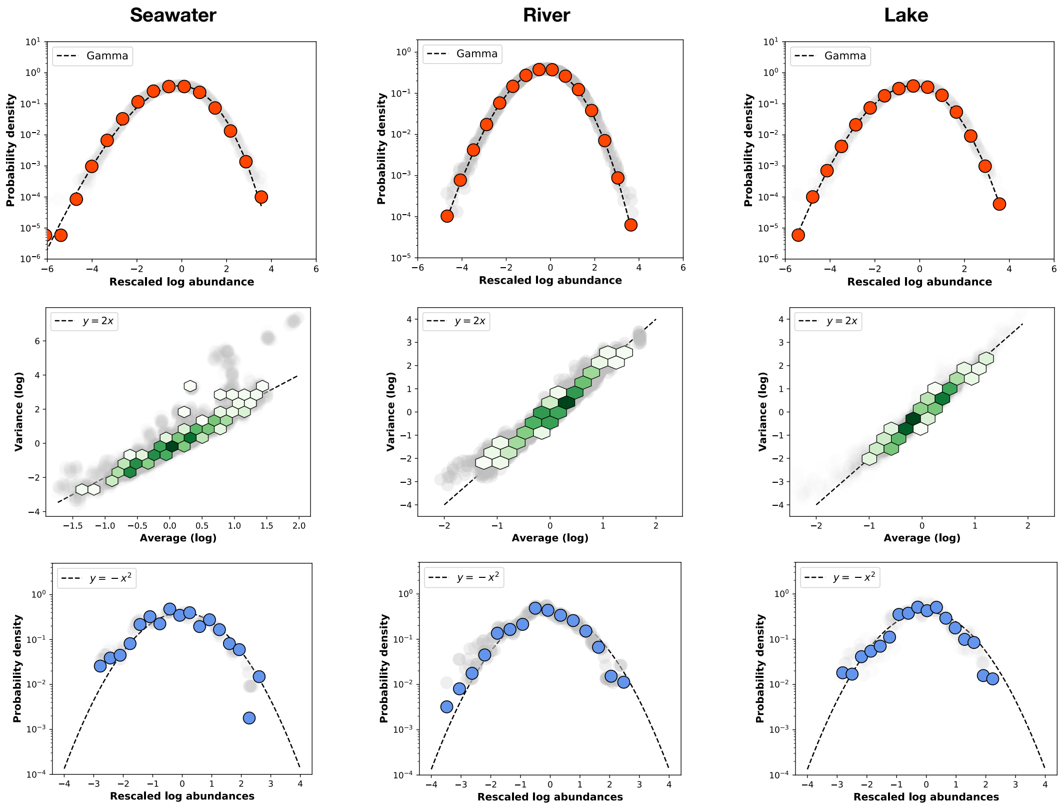


Figure S16: **Three macroecological laws for *in-silico* communities generated through MCMC**. From top to bottom, the abundance fluctuation distribution, Taylor's law, and the mean abundance distribution of *in-silico* communities, as obtained by fitting the abundance correlation distribution through the MCMC algorithm presented in the main text. Biomes analyzed in this plot, from left to right: *Seawater*, *River*, and *Lake*.

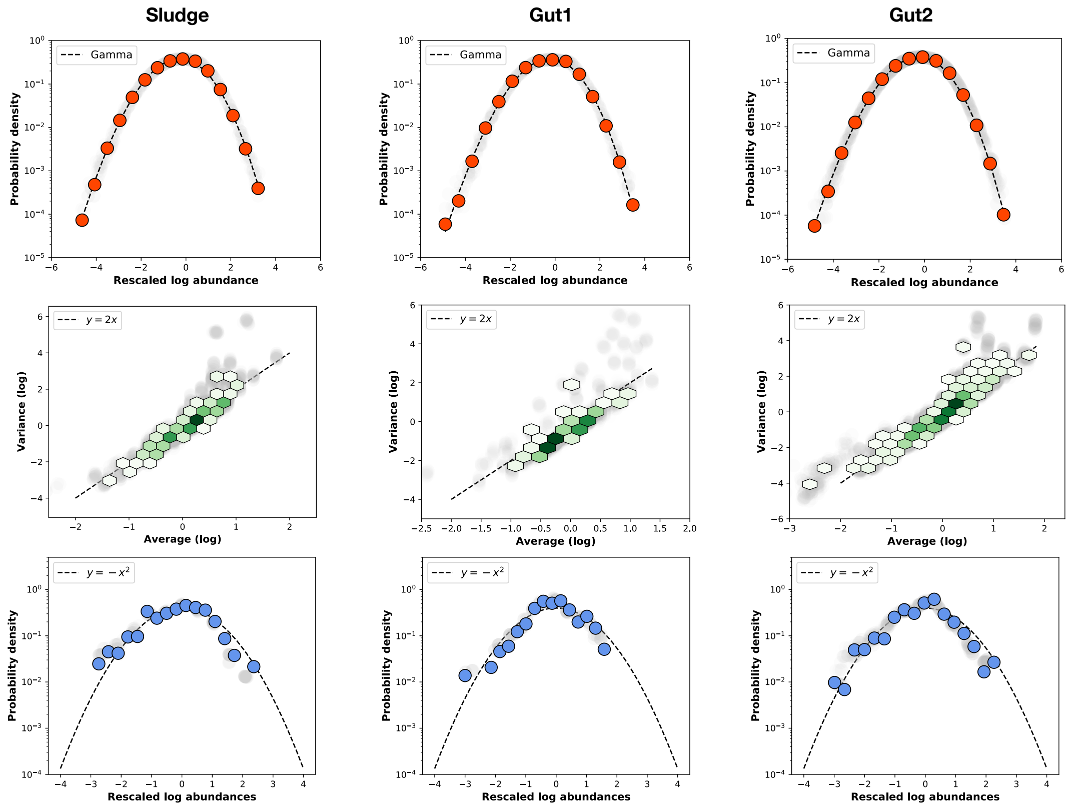


Figure S17: **Three macroecological laws for *in-silico* communities generated through MCMC**. From top to bottom, the abundance fluctuation distribution, Taylor's law, and the mean abundance distribution of *in-silico* communities, as obtained by fitting the abundance correlation distribution through the MCMC algorithm presented in the main text. Biomes analyzed in this plot, from left to right: *Sludge*, *Gut1*, and *Gut2*).

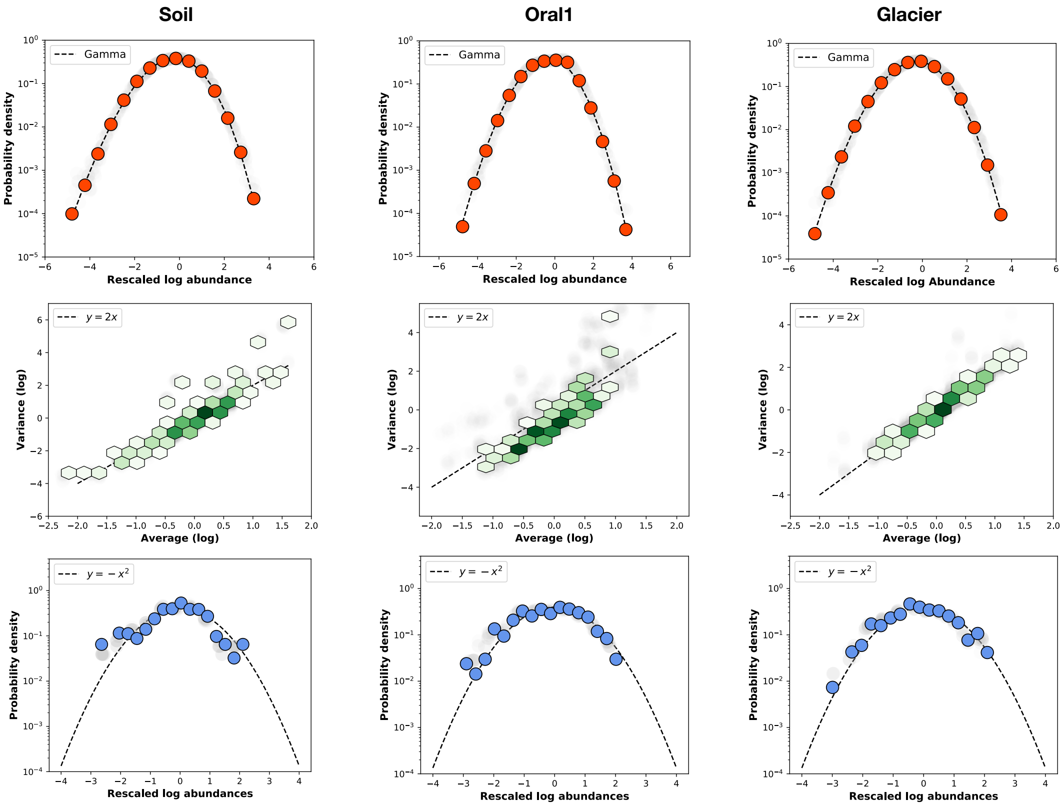


Figure S18: **Three macroecological laws for *in-silico* communities generated through MCMC**. From top to bottom, the abundance fluctuation distribution, Taylor's law, and the mean abundance distribution of *in-silico* communities, as obtained by fitting the abundance correlation distribution through the MCMC algorithm presented in the main text. Biomes analyzed in this plot, from left to right: *Soil*, *Oral1*, and *Glacier*.

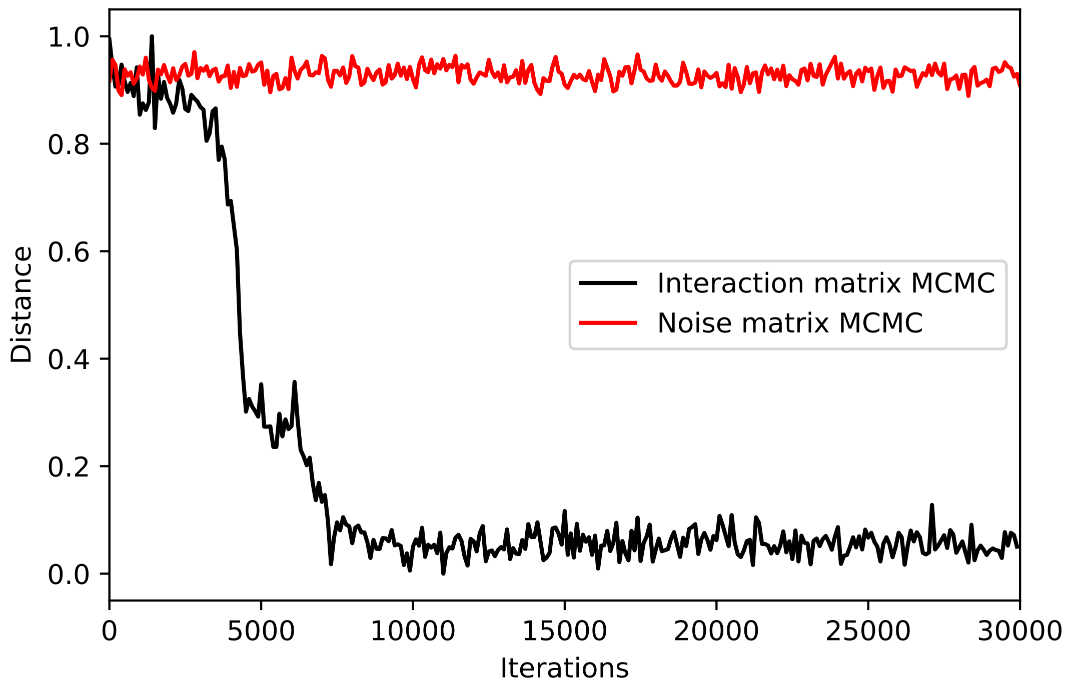


Figure S19: **Distance from the logarithm of the generated correlation distribution to the empirical one, in a typical run of the MCMC, as applied to the interaction matrix A (black) or to the noise matrix W (red).** Biome: Seawater

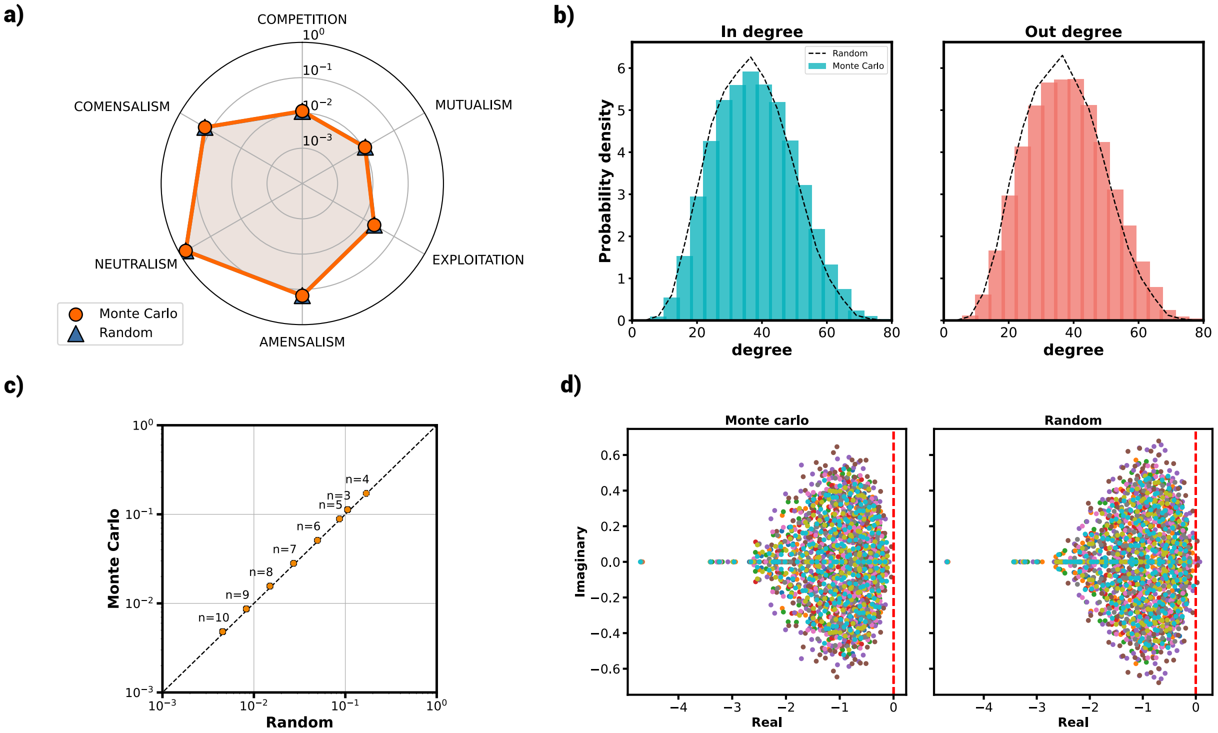


Figure S20: **Statistical Properties of Monte Carlo matrices vs. Random one** The figure displays the (log of the) fraction of interaction types **(a)**; in-degree distribution (left panel) and out-degree distribution (right panel) **(b)**; number of loops of order $n$ **(c)**; and spectral density for 10 typical matrices (each color corresponding to a different matrix) **(d)**. These patterns represent the averages over a set of 200 matrices obtained through the MCMC method, minimizing the correlation distribution and Grilli's laws, for the *Seawater* biome with $o = 0.5$. These properties are compared against an ensemble of random matrices, where the weights are sampled from a Gaussian distribution with a mean value of zero and standard deviations matching those of the MCMC matrices. Connectivity is also set according to that of the matrices taken from MCMC. The size is determined by the biome $S = 199$.

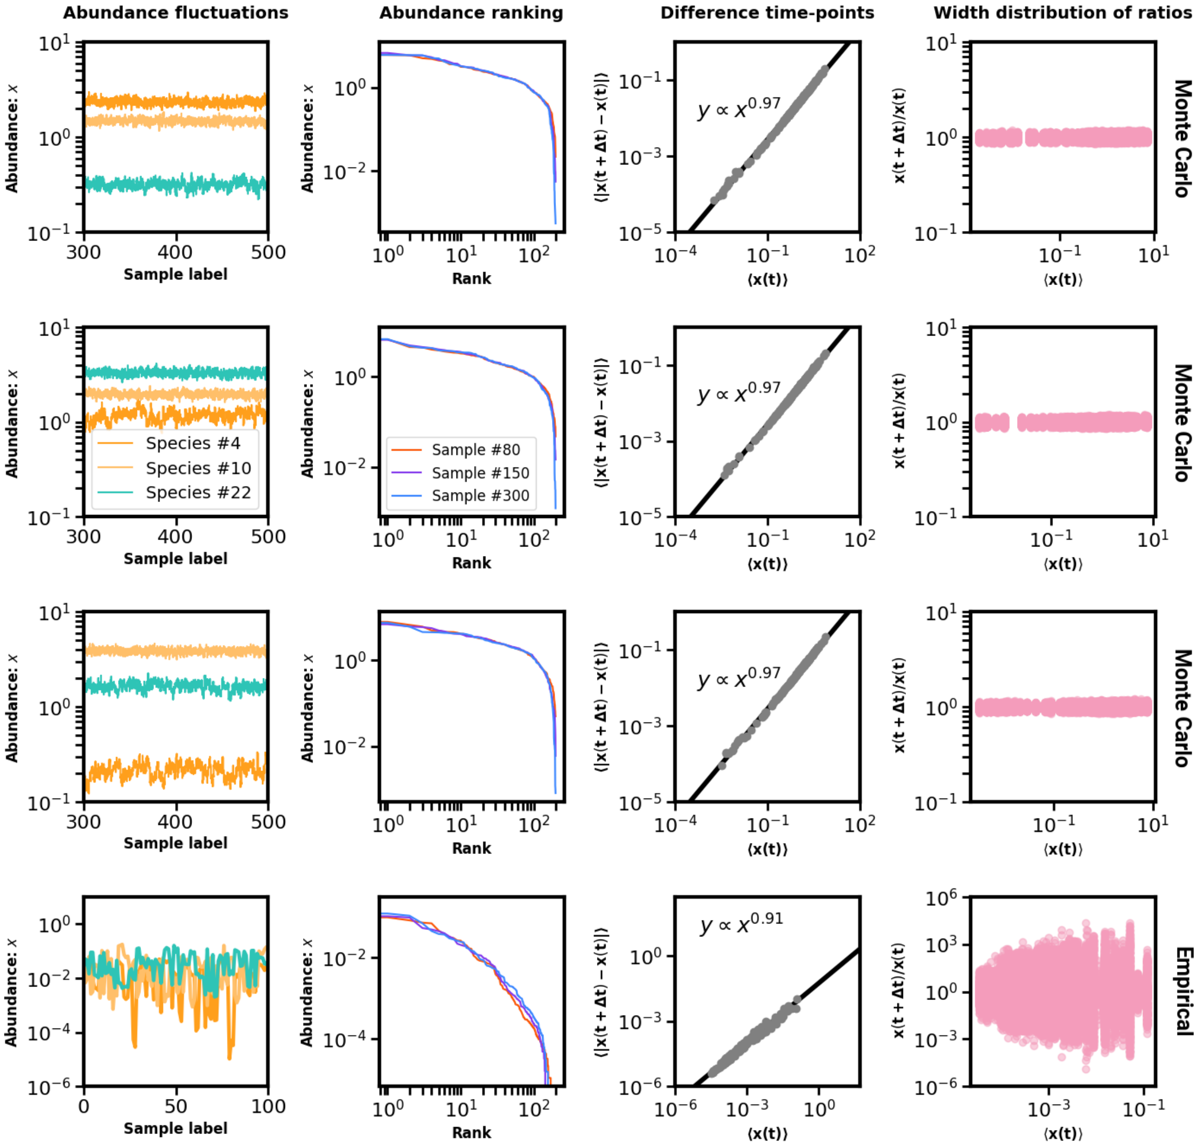


Figure S21: **Descheemaeker's macroecological properties for different population model**. The rows in the matrix correspond to randomly selected MCMC-generated matrices from those studied in Fig. S20, while the columns represent patterns examined in [9]. In detail, the first column illustrates abundance fluctuations for three random species. The second column displays the rank of abundances, with different lines corresponding to different (random) samples (i.e., time instants). Notably, all lines exhibit the same behavior, where the rank of abundances remains stable over time, resembling a marked heavy-tailed character. Moving on to the third column, it explores the average distance between abundances at consecutive time points, $\langle |x(t + \Delta t) - x(t)| \rangle$. The dependence on the mean abundance $\langle x(t) \rangle$ shows a linear behavior (in log-log scale), a consequence of the linear nature of noise. Lastly, the fourth column depicts the abundance ratio at two consecutive time points $x(t + \Delta t)/x(t)$, which is independent of the mean abundance. The Stochastic Lotka-Volterra dynamics were run with the same parameters considered in Fig. 4. Upon visual inspection, the model reproduces the patterns unveiled in [9] quite accurately. For third and fourth columns the time step been taken equal to the integration step: $\Delta t = h = 0.01$.

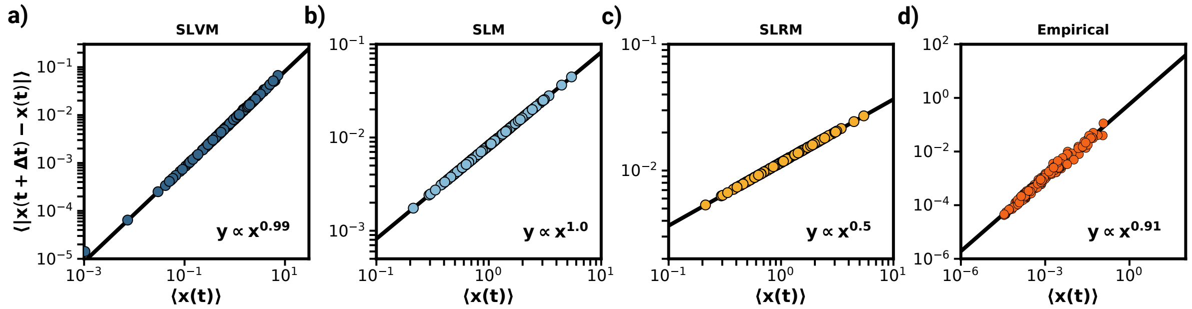


Figure S22: **Average shift of abundances for different population models**. The average difference in species abundance between different time points has been observed to exhibit a linear dependence on the mean abundance [9]. The resulting slope offers insights into the magnitude of the shift. In this context, we illustrate this pattern for various population models: the Stochastic Lotka-Volterra model (SLVM) in Eq. (S1) (**a**), the Stochastic Logistic model from [2] (**b**), the Stochastic Linear Response model (SLRM) introduced in [10] (**c**), and the empirical data for the Seawater biome (**d**). Notably, both SLM and SLVM exhibit slopes in line with empirical data ($y/x \approx 1$), while the prediction of SLRM deviates noticeably. The SLVM dynamics is runned with the same parameters of Fig. 4 in the main text and the interaction matrices generated by the MCMC and studied in Fig. S20. The SLM is simulated with the same $K_i$s of the interaction matrix generated by the MCMC, and the SLRM has been simulated using those carrying capacities to set $x_i^\star = K_i$. Finally in all panels the time step been taken equal to the integration step: $\Delta t = h = 0.01$.
